# Supplementary material for: Chirality-Induced Selectivity of Phonon Angular Momenta in Chiral Quartz Crystals
Source: arXiv:2401.17158 ancillary file (2024-01-30)
Supplement: Supplementary file 1 [file heatCISSarXiv_Supplemental.pdf]

# Supplemental Materials for
# "Chirality-Induced Selectivity of Phonon Angular Momenta in Chiral Quartz Crystals"

Kazuki Ohe[1], Hiroaki Shishido[1,2], Masaki Kato[3], Shoyo Utsumi[2],
Hiroyasu Matsuura[3], and Yoshihiko Togawa[1,2,4]*

[1]*Department of Physics and Electronics, Osaka Prefecture University,*
*1-1 Gakuencho, Sakai, Osaka 599-8531, Japan*

[2]*Department of Physics and Electronics, Osaka Metroplitan University,*
*1-1 Gakuencho, Sakai, Osaka 599-8531, Japan*

[3]*Department of Physics, The University of Tokyo, Bunkyo, Tokyo 113-0033, Japan and*

[4]*Quantum Research Center for Chirality,*
*Institute for Molecular Science, Okazaki 444-8585, Japan*

(Dated: Received 8 April 2022, Revised 5 November 2022, 18 October 2023.)

## CONTENTS

1. Experimental setup for thermal transport measurements at cryogenic temperatures 2

2. Experiment using an achiral substrate of magnesium oxide 4

3. Experiment for spin injection from electrode into quartz 5

4. Theoretical analysis 6
   Lattice vibration 6
   Hamiltonian 6
   Phonon angular momentum 7
   Boltzmann equation 7

5. Definition of the handedness of $\alpha$-quartz 10

References 11

## 1. EXPERIMENTAL SETUP FOR THERMAL TRANSPORT MEASUREMENTS AT CRYOGENIC TEMPERATURES

In the device designed for thermal transport measurements, which follows that for the conventional thermal measurements performed at cryogenic temperatures [1–3], the quartz substrate stands up on a heat bath made of copper with a trench for thermal contact, while a tip resistor is put on the top surface of the substrate as an electrical heater, as shown in Fig. S1. For enhancing a thermal contact between them, the quartz substrate is attached to the heat bath via silver paste, while the heater is fixed to the quartz by using varnish. The thermal resistance of the lead wires is much higher than that of the quartz substrate, and thus the heat leak through the lead wires is negligibly small. This configuration guarantees an introduction of temperature gradient and thus a unidirectional heat flow from the top surface to the bottom one of the quartz substrate. The temperature gradient was estimated using a thermal conductivity of $\alpha$ quartz.

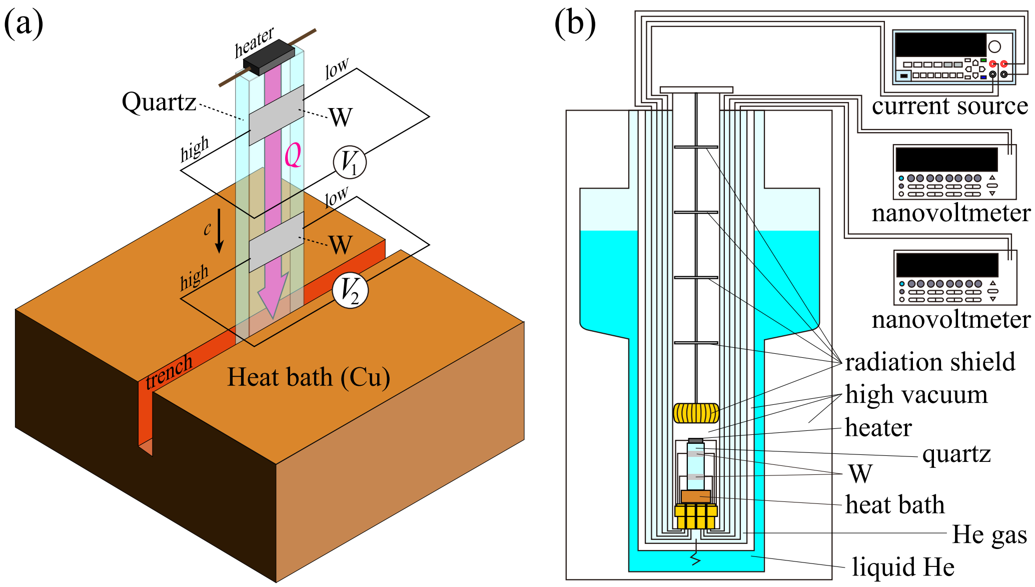


FIG. S1. Experimental setup for thermal transport measurements.

Thermal convection and radiation should be suppressed when performing thermal measurements. In the present experimental setup, the thermal convection is caused by gases around the substrate. The thermal radiation, which is generated in proportion to a difference of the fourth power of temperatures at the thermal source and thermally radiated object, may induce a temperature difference between both sides of the detection electrode and an extrinsic voltage signal due to a thermoelectromotive force along it. Thus, the experiments were performed at a vacuum

condition of $10^{-3}$ Pa at low temperatures so as to reduce artefacts caused by heat leak, thermal convection, and radiation as much as possible. For instance, the thermal radiation was estimated to be less than 20 nW at 10 K and 60 μW at 40 K. In this condition, the heat introduced by the tip resistor is expected to flow along the quartz.

In the measurements, first, the temperature is set to be constant at the heat bath, which is cooled by gaseous helium. Then, the constant current is applied to the tip resistor and a voltage generated across it is monitored for calculating an injected thermal power. After the temperature gradient becomes steady, the transverse voltage signals are simultaneously measured in the detection electrodes as a function of the thermal power.

## 2. EXPERIMENT USING AN ACHIRAL SUBSTRATE OF MAGNESIUM OXIDE

A control experiment was conducted in the same measurement setup (shown in Fig. S1) with a magnesium oxide (MgO) substrate. Figure. S2 shows the conversion coefficient $A$ of the signal as a function of temperature. No signal appears in the measured temperature regime in the achiral (non-chiral) MgO substrate with the tungsten (W) electrodes.

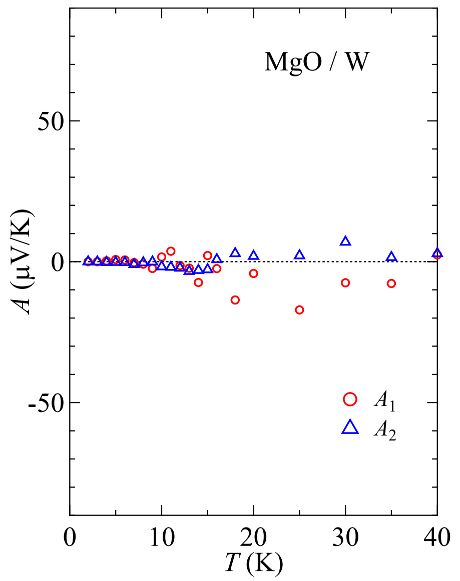


FIG. S2. The conversion coefficient $A$ of the signal as a function of temperature with a MgO substrate with the W electrodes.

### 3. EXPERIMENT FOR SPIN INJECTION FROM ELECTRODE INTO QUARTZ

Using the same devices (without the tip resistor), a spin injection from the transverse electrode into the chiral quartz via a spin Hall effect [4, 5] was examined. In the present experiment, while the current was applied to the electrode on the upper side of the quartz, the voltage signal was detected on the other electrode on the lower side of quartz. An asymmetric behavior was found in the current-voltage characteristics, as shown in Fig. S3(a). Even and odd components were extracted with regard to the strength of the applied current. The even component is clearly seen in the current-voltage characteristics, while the odd component is hardly found, as shown in Fig. S3(b), suggesting that the observed voltage was generated by a thermally driven conversion process in the chiral quartz. These data are consistent with that observed in Figs. 1 and 2 in the main text and also support that the generation, propagation, and transfer of spin angular momenta could occur in the chiral quartz under the thermal flow. Indeed, even in this experimental setup, the signal sign reverses in the quartz substrate with the opposite handedness.

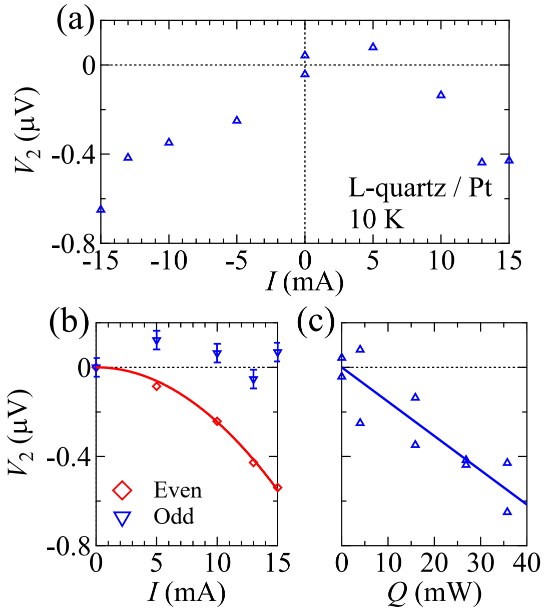


FIG. S3. (a) Current-voltage characteristics obtained in the experimental setup for the spin injection from electrode into quartz. (b) Even and odd components of the data. (c) The data replotted as a function of the input thermal power $Q$.

## 4. THEORETICAL ANALYSIS

In this section, we provide the theoretical calculations of thermal transport coefficients of $\alpha$-quartz, associated with the chiral phonons [6, 7].

### Lattice vibration

Initially, we formulate lattice vibration in a general manner by following textbooks [8]. When there are $M$ atoms in each unit cell, the position of the $b$-th atom in the $l$-th unit cell can be written as $\boldsymbol{R}_{lb}^{(0)} = \boldsymbol{R}_l + \boldsymbol{r}_b$ in equilibrium, where $\boldsymbol{R}_l$ and $\boldsymbol{r}_b$ denote the position of the $l$-th unit cell and the $b$-th atom from the unit cell position, respectively.

If we assume an interatomic Coulomb potential $V$ and consider up to the second order terms with respect to the displacement, the Euler-Lagrange equation for the displacement vector of the $b$-th atom in the $l$-th unit cell $\boldsymbol{u}_{lb}$ becomes

$$m_b \ddot{u}_{lb}^{\alpha} + \sum_{l'b'} \sum_{\beta} V_{lbl'b'}^{\alpha\beta} u_{l'b'}^{\beta} = 0, \tag{1}$$

where $V_{lbl'b'}^{\alpha\beta} = \left. \frac{\partial^2 V}{\partial u_{lb}^{\alpha} \partial u_{l'b'}^{\beta}} \right|_{u=0}$ and $m_b$ denotes the mass of the $b$-th atom.

Substituting a plane wave solution $\boldsymbol{u}_{lb} = \frac{1}{\sqrt{m_b}} \boldsymbol{e}_{\boldsymbol{q}bp} e^{i(\boldsymbol{q}\cdot\boldsymbol{R}_l - \omega_{\boldsymbol{q}p} t)}$ into eq.(1), the kinetic equation becomes

$$\omega_{\boldsymbol{q}p}^2 e_{\boldsymbol{q}bp}^{\alpha} - \sum_{b'} \sum_{\beta} D_{bb'}^{\alpha\beta}(\boldsymbol{q}) e_{\boldsymbol{q}b'p}^{\beta} = 0, \tag{2}$$

where $\boldsymbol{e}_{\boldsymbol{q}bp}$ is a normalized eigenvector corresponding to the $p$-th eigenvalue with the wave vector $\boldsymbol{q}$, $\omega_{\boldsymbol{q}p}^2$, and $D_{bb'}^{\alpha\beta}(\boldsymbol{q}) = \sum_{l-l'} \frac{V_{lbl'b'}^{\alpha\beta}}{\sqrt{m_b m_{b'}}} e^{-i\boldsymbol{q}\cdot(\boldsymbol{R}_l - \boldsymbol{R}_{l'})}$ is called a dynamical matrix. To parametrize the dynamical matrix of $\alpha$-quartz, we restrict the range of the interactions to the second nearest neighbors. Additionally we regard the $SiO_4$ tetrahedra as regular tetrahedra and impose this local symmetry on the dynamical matrix [9]. As a result, we can reduce the number of the parameters to six and they were determined so that the dispersion matched that obtained in the previous study [9].

### Hamiltonian

The Hamiltonian describing the lattice vibration can be written as

$$\mathcal{H} = \sum_{lb} \sum_{\alpha} \frac{P_{lb}^{\alpha} P_{lb}^{\alpha}}{2m_b} + \frac{1}{2} \sum_{lbl'b'} \sum_{\alpha\beta} u_{lb}^{\alpha} V_{lbl'b'}^{\alpha\beta} u_{l'b'}^{\beta}, \tag{3}$$

where $\boldsymbol{P}_{lb}$ is the momentum of the $b$-th atom in the $l$-th unit cell. Using the Fourier transformations $u_{lb}^{\alpha} = \frac{1}{\sqrt{N}}\sum_{\boldsymbol{q}} e^{i\boldsymbol{q}\cdot\boldsymbol{R}_l} u_{\boldsymbol{q}b}^{\alpha}$ and $P_{lb}^{\alpha} = \frac{1}{\sqrt{N}}\sum_{\boldsymbol{q}} e^{-i\boldsymbol{q}\cdot\boldsymbol{R}_l} P_{\boldsymbol{q}b}^{\alpha}$ followed by the variable transformations $\tilde{u}_{\boldsymbol{q}p} = \sum_b \sqrt{m_b}\boldsymbol{e}_{\boldsymbol{q}bp}^* \cdot \boldsymbol{u}_{\boldsymbol{q}b}$ and $\tilde{P}_{\boldsymbol{q}p} = \sum_b \frac{1}{\sqrt{m_b}}\boldsymbol{e}_{\boldsymbol{q}bp} \cdot \boldsymbol{P}_{\boldsymbol{q}b}$, the Hamiltonian becomes

$$\mathcal{H} = \frac{1}{2}\sum_{\boldsymbol{q}p} \tilde{P}_{\boldsymbol{q}b}\tilde{P}_{\boldsymbol{q}b}^* + \frac{1}{2}\sum_{\boldsymbol{q}p} \omega_{\boldsymbol{q}p}^2 \tilde{u}_{\boldsymbol{q}b}\tilde{u}_{\boldsymbol{q}b}^*. \tag{4}$$

Introducing the annihilation and creation operators of phonons defined by $a_{-\boldsymbol{q}p} = \frac{i}{\sqrt{2\hbar\omega_{\boldsymbol{q}p}}}\tilde{P}_{\boldsymbol{q}p} + \sqrt{\frac{\omega_{\boldsymbol{q}p}}{2\hbar}}\tilde{u}_{\boldsymbol{q}p}$ and $a_{\boldsymbol{q}p}^{\dagger} = \frac{1}{i\sqrt{2\hbar\omega_{\boldsymbol{q}p}}}\tilde{P}_{\boldsymbol{q}p} + \sqrt{\frac{\omega_{\boldsymbol{q}p}}{2\hbar}}\tilde{u}_{\boldsymbol{q}p}$, the Hamiltonian is quantized in a well-known form:

$$\mathcal{H} = \hbar\omega_{\boldsymbol{q}p}\left(a_{\boldsymbol{q}p}^{\dagger}a_{\boldsymbol{q}p} + \frac{1}{2}\right). \tag{5}$$

**Phonon angular momentum**

The phonon angular momentum is defined as the orbital angular momentum of the atoms:

$$\boldsymbol{L} = \frac{1}{V}\sum_{lb} \boldsymbol{u}_{lb}(t) \times m_b\dot{\boldsymbol{u}}_{lb}(t). \tag{6}$$

Here we used the Heisenberg picture for operators. Expressing $\boldsymbol{L}$ in terms of the creation and annihilation operators and then neglecting the terms rapidly oscillating in time [10], we obtain

$$\boldsymbol{L} = \frac{i\hbar}{V}\sum_{b}\sum_{\boldsymbol{q}pp'} \boldsymbol{e}_{\boldsymbol{q}bp} \times \boldsymbol{e}_{\boldsymbol{q}bp'}^* \left(a_{\boldsymbol{q}p}^{\dagger}a_{\boldsymbol{q}p'} + \frac{1}{2}\delta_{pp'}\right) e^{-i(\omega_{\boldsymbol{q}p}-\omega_{\boldsymbol{q}p'})t}. \tag{7}$$

By using the fact that $\langle a_{\boldsymbol{q}p}^{\dagger}a_{\boldsymbol{q}p}\rangle = n_0(\omega_{\boldsymbol{q}p})\delta_{pp'}$ holds in equilibrium [10], the phonon angular momentum can be written as

$$\boldsymbol{L}_{\mathrm{eq}} = \frac{1}{V}\sum_{\boldsymbol{q}p} \boldsymbol{\ell}_{\boldsymbol{q}p}\left(n_0(\omega_{\boldsymbol{q}p}) + \frac{1}{2}\right), \tag{8}$$

$$\boldsymbol{\ell}_{\boldsymbol{q}p} = i\hbar\sum_{b} \boldsymbol{e}_{\boldsymbol{q}bp} \times \boldsymbol{e}_{\boldsymbol{q}bp}^*, \tag{9}$$

where $n_0(\omega) = \frac{1}{e^{\beta\hbar\omega}-1}$ is the Bose distribution function and $\beta$ is the inverse temperature.

**Boltzmann equation**

When temperature gradient is applied to a phonon system, the distribution function shifts from the equilibrium one. The deviation can be described by the Boltzmann equation with relaxation time approximation :

$$n(\omega_{\boldsymbol{q}p}) - n_0(\omega_{\boldsymbol{q}p}) = \tau_{\boldsymbol{q}p}\left[\boldsymbol{v}_{\boldsymbol{q}p}\cdot\left(-\frac{\hbar\omega_{\boldsymbol{q}p}}{T}\frac{\partial n_0}{\partial\hbar\omega_{\boldsymbol{q}p}}\boldsymbol{\nabla}T\right)\right], \tag{10}$$

where $n(\omega)$ denotes the non-equilibrium distribution function of phonons, $\tau_{\boldsymbol{q}p}$ is the relaxation time, $\boldsymbol{v}_{\boldsymbol{q}p}$ is the velocity of phonons, and $T$ is the temperature.

By substituting this expression into the heat current of phonons $J_{\mathrm{Q}}^{z} = \frac{1}{V}\sum_{\boldsymbol{q}p}\hbar\omega_{\boldsymbol{q}p}v_{\boldsymbol{q}p}^{z}n(\omega_{\boldsymbol{q}p})$, we obtain the thermal conductivity along the $c$-axis:

$$\kappa = \frac{1}{VT}\sum_{\boldsymbol{q}p}(\hbar\omega_{\boldsymbol{q}p})^2(v_{\boldsymbol{q}p}^{z})^2\tau_{\boldsymbol{q}p}\left(-\frac{\partial n_0}{\partial\hbar\omega_{\boldsymbol{q}p}}\right) \tag{11}$$

$$= \frac{1}{T}\sum_{p}\int d\epsilon D_p(\epsilon)\tau_p(\epsilon/\hbar)\epsilon^2\left(-\frac{\partial n_0}{\partial\epsilon}\right), \tag{12}$$

where $V$ is the volume of the lattice and $D_p(\epsilon) = \frac{1}{V}\sum_{\boldsymbol{q}}(v_{\boldsymbol{q}p}^{z})^2\delta(\epsilon - \hbar\omega_{\boldsymbol{q}p})$. In the second line, we approximated that the relaxation time depended only on the branch and the frequency.

Following the same steps, we can obtain the thermal angular momentum coefficient $\kappa_{\mathrm{AM}}$ defined by $L^z = \kappa_{\mathrm{AM}}(-\nabla_z T)$ [11]. By replacing $n_0(\omega_{\boldsymbol{q}p})$ with $n(\omega_{\boldsymbol{q}p})$ in eq.(8) and using eq.(10), we obtain

$$\kappa_{\mathrm{AM}} = \frac{1}{VT}\sum_{\boldsymbol{q}p}\hbar\omega_{\boldsymbol{q}p}\hbar\ell_{\boldsymbol{q}p}^{z}v_{\boldsymbol{q}p}^{z}\tau_{\boldsymbol{q}p}\left(-\frac{\partial n_0}{\partial\hbar\omega_{\boldsymbol{q}p}}\right) \tag{13}$$

$$= \frac{1}{T}\sum_{p}\int d\epsilon\tilde{D}_p(\epsilon)\tau_p(\epsilon/\hbar)\epsilon\left(-\frac{\partial n_0}{\partial\epsilon}\right), \tag{14}$$

where $\tilde{D}_p(\epsilon) = \frac{1}{V}\sum_{\boldsymbol{q}}\delta(\epsilon - \hbar\omega_{\boldsymbol{q}p})\hbar\ell_{\boldsymbol{q}p}^{z}v_{\boldsymbol{q}p}^{z}$. In the numerical calculations, the tetrahedron method was used to calculate $D_p(\epsilon)$ and $\tilde{D}_p(\epsilon)$ with high precision [12].

In this letter, we use the following relaxation time [13, 14]:

$$\tau_p^{-1}(\omega) = \tau_{\mathrm{B}}^{-1} + \tau_{\mathrm{I}}^{-1} + \tau_{\mathrm{U}}^{-1} \tag{15}$$

$$= \frac{\bar{v}_p(\omega)}{L} + A\omega^4 + B\omega^2 T\exp\left(-\frac{\Theta_{\mathrm{D}}}{3T}\right). \tag{16}$$

The first term represents the size effect or boundary scattering. $\bar{v}_p(\omega) = \frac{1}{V\rho(\omega)}\sum_{\boldsymbol{q}}\left|\frac{\partial\omega_{\boldsymbol{q}p}}{\partial\boldsymbol{q}}\right|\delta(\omega - \omega_{\boldsymbol{q}p})$ denotes the average velocity of the branch $p$, where $\rho_p(\omega) = \frac{1}{V}\sum_{\boldsymbol{q}}\delta(\omega - \omega_{\boldsymbol{q}p})$ is the density of states, and $L$ denotes the system length. The second and third terms represent scattering by point defects and the Umklapp process of phonon-phonon scattering, respectively, where $\Theta_{\mathrm{D}}$ is the Debye temperature.

The parameters were determined so as to reproduce the thermal conductivity measured in the experiment. We set $A = 9.3\times10^{-43}\,\mathrm{s}^3$, $B = 2.0\times10^{-17}\,\mathrm{s/K}$, $L = 10\,\mathrm{mm}$ and $\Theta_{\mathrm{D}} = 200\,\mathrm{K}$. Since the Debye temperature depends on the branch in general, we used a branch-independent single value.

There are different choices for the approximated relaxation time, e.g. an additional term for the normal process scattering $\tau_{\mathrm{N}}^{-1} = B_1\omega^2T^3$ and an alternative expression for the Umklapp process $\tau_{\mathrm{U}}^{-1} = B_2\omega^2T^3e^{-\Theta_{\mathrm{D}}/(\alpha T)}$ [14–17]. We confirmed that there was a good parameter set for this

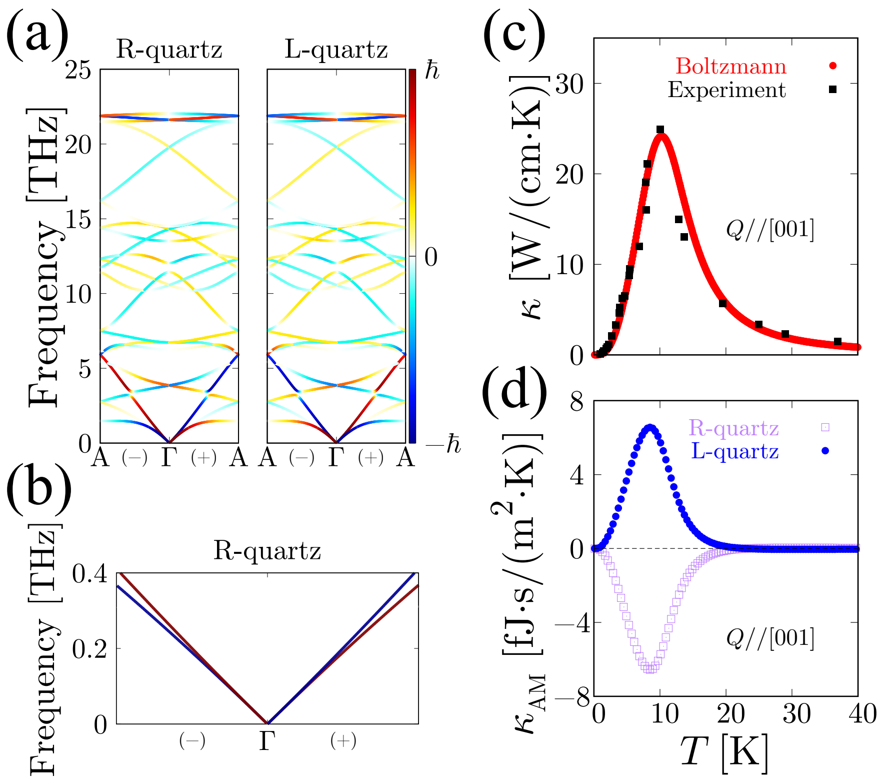


FIG. S4. Analytical calculations of phonon dispersion (a and b), thermal conductivity (c), and propagation of net angular momenta (d) for $\alpha$ quartz. The data of thermal conductivity of $\alpha$ quartz is derived from that in the literature [18].

combination of relaxation times and that it gave a similar result of thermal angular momentum coefficient.

The phonon dispersion of $\alpha$-quartz is shown in Fig. S4(a). A split of the phonon branches is clearly found in the vicinity of $\Gamma$ point along the $\Gamma - A$ line in Fig. S4(b). Importantly, two of the phonon branches carry the angular momenta with the opposite sign. The sign depends on the handedness of the quartz.

Figures S4(c) and S4(d) shows the analytical calculation of thermal conductivity and the net angular momenta carried by thermally-driven phonons at a finite temperature, respectively. A peak structure appears at around 10 K in a temperature dependence of the coefficient for the angular momenta propagation. This result is quite consistent with the experimental data in Fig. 2 in the main text.

## 5. DEFINITION OF THE HANDEDNESS OF $\alpha$-QUARTZ

As for the handedness of $\alpha$-quartz [19, 20], some confusing descriptions are found in the literature. In the present study, we use the definition based on the crystallographic structure of atoms [19], as shown in Table. SI. The $\alpha$-quartz crystal that belongs to the space group of $P3_121$ has a right-handed helical structure of $SiO_4$ tetrahedrons, while the one for $P3_221$ has a left-handed helical one. Here, according to these atomic structures of crystals, the former crystal is called R-quartz and the latter is L-quartz. Note that this definition is opposite to that determined by the optical activity. The latter definition is generally adopted in the industrial use [20].

TABLE I. The definition of the handedness of $\alpha$-quartz.

| $\alpha$-quartz | | |
|---|---|---|
| Helical structure of $SiO_4$ | right-handed helix | left-handed helix |
| Space group | $P3_121$ | $P3_221$ |
| Name used in this study | R-quartz | L-quartz |
| Optical rotation (O.R.) | anti-clockwise (levo-rotatory) | clockwise (dextro-rotatory) |
| Name from O.R. | (-)-quartz (l-quartz) | (+)-quartz (d-quartz) |
| Name in industrial use | L-quartz | R-quartz |

---

* ytogawa@omu.ac.jp

[1] G. A. Slack, Effect of Isotopes on Low-Temperature Thermal Conductivity, Phys. Rev. **105**, 829 (1957).

[2] G. A. Slack, Thermal Conductivity of $CaF_2$, $MnF_2$, $CoF_2$, and $ZnF_2$ Crystals, Phys. Rev. **122**, 1451 (1961).

[3] G. K. White, *Experimental Techniques in Low Temperature Physics* (3rd edn., Oxford University Press, U.S., 1979), Ch. VII, 171.

[4] T. Kimura, Y. Otani, T. Sato, S. Takahashi, and S. Maekawa, Room-temperature reversible spin Hall effect, Phys. Rev. Lett. **98**, 156601 (2007).

[5] A. Inui, R. Aoki, Y. Nishiue, K. Shiota, Y. Kousaka, H. Shishido, D. Hirobe, M. Suda, J. Ohe, J. Kishine, H. M. Yamamoto, and Y. Togawa, Chirality-Induced Spin-Polarized State of a Chiral Crystal $CrNb_3S_6$, Phys. Rev. Lett. **124**, 166602 (2020).

[6] J. Kishine, A. S. Ovchinnikov, and A. A. Tereshchenko, Chirality-Induced Phonon Dispersion in a Noncentrosymmetric Micropolar Crystal, Phys. Rev. Lett. **125**, 245302 (2020).

[7] K. Ishito, H. Mao, Y. Kousaka, Y. Togawa, S. Iwasaki, T. Zhang, S. Murakami, J. Kishine, and T. Satoh, Truly chiral phonons in $\alpha$-HgS, Nat. Phys. **19**, 35 (2023).

[8] J. M. Ziman, *Electrons and phonons: the theory of transport phenomena in solids* (Oxford University Press, U.S., 2001).

[9] M. M. Elcombe, Some aspects of the lattice dynamics of quartz, Proc. Phys. Soc. **91**, 947 (1967).

[10] L. Zhang and Q. Niu, Angular Momentum of Phonons and the Einstein–de Haas Effect, Phys. Rev. Lett. **112**, 085503 (2014).

[11] M. Hamada, E. Minamitani, M. Hirayama, and S. Murakami, Phonon Angular Momentum Induced by the Temperature Gradient, Phys. Rev. Lett. **121**, 175301 (2018).

[12] O. Jepson and O. K. Anderson, The electronic structure of h.c.p. Ytterbium, Solid State Commun. **9**, 1763 (1971).

[13] Y. Li, T. Zhang, Y. Qin, T. Day, G. J. Snyder, X. Shi, and L. Chen, Thermoelectric transport properties of diamond-like $Cu_{1-x}Fe_{1+x}S_2$ tetrahedral compounds, J. Appl. Phys. **116**, 203705 (2014).

[14] B. Singh, M. Roy, V. Menon, and K. Sood, Effects of dispersion, correction term, and isotopes on the thermal conductivity of LiF crystal, Phys. Rev. B **67**, 014302 (2003).

[15] M. G. Holland, Analysis of Lattice Thermal Conductivity, Phys. Rev. **132**, 2461 (1963).

[16] Y. P. Joshi and G. S. Verma, Analysis of Phonon Conductivity: Application to Si, Phys. Rev. B **1**, 750 (1970).

[17] A. C. Sparavigna, The Boltzmann Equation of Phonon Thermal Transport Solved in the Relaxation Time Approximation – II – Data Analysis, Mech. Mater. Sci. Eng. J. **2016**, 57 (2016).

[18] R. C. Zeller and R. O. Pohl, Thermal Conductivity and Specific Heat of Noncrystalline Solids, Phys. Rev. B **4**, 2029 (1971).

[19] A. M. Glazer and K. Stadnikca, On the origin of optical activity in crystal structures, J. Appl. Crystallogr. **19**, 108 (1986).

[20] Y. Tanaka, T. Takeuchi, S. W. Lovesey, K. S. Knight, A. Chainani, Y. Takata, M. Oura, Y. Senba, H. Ohashi, and S. Shin, Right Handed or Left Handed? Forbidden X-Ray Diffraction Reveals Chirality, Phys. Rev. Lett. **100**, 145502 (2008).
